# Supplementary material for: Automatic Completion of Distributed Protocols with Symmetry
Source: arXiv:1505.04409 source file (2015-05-17)
Supplement: Supplementary file 1 [file appendix.tex]

%!TEX root = cav15.tex
